# Supplementary material for: Adaptively-Realistic Image Generation from Stroke and Sketch with Diffusion Model
Source: arXiv:2208.12675 source file (2022-09-01)
Supplement: Supplementary file 1 [file supp-s2i-comp.tex]

\begin{figure*}[t!]
    \centering
    
    \setlength\tabcolsep{1.5pt} % default value: 6pt
    \begin{tabular}{ccc c:c cccc}
    Sketch & Stroke & Combine &  &  & Ours & SDEdit~\cite{meng2021sdedit} & SSS2IS~\cite{liu2021self} & U-GAT-IT~\cite{kim2019u} \\
    \includegraphics[height=.4\linewidth]{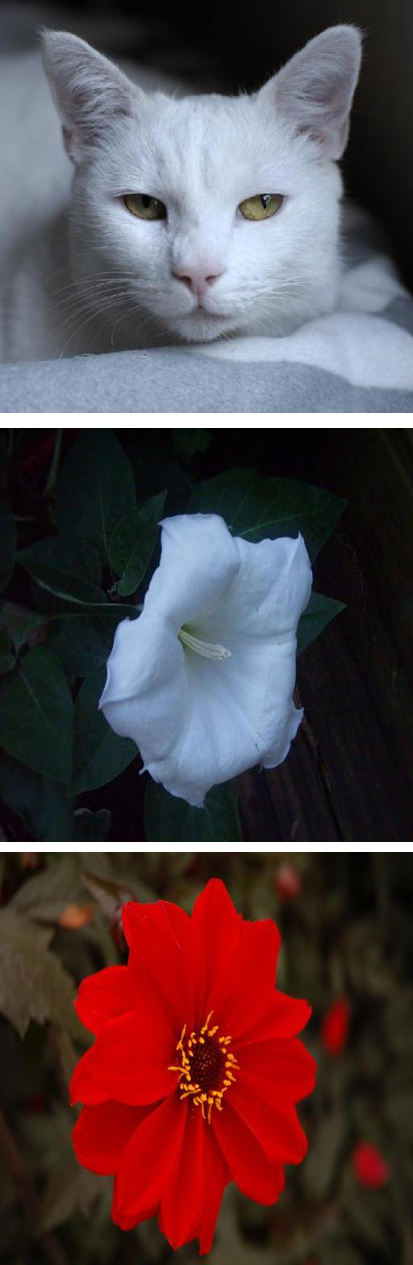} &
    \includegraphics[height=.4\linewidth]{tex/images/app-left-original.png} &
    \includegraphics[height=.4\linewidth]{tex/images/app-left-original.png} & & &
    \includegraphics[height=.4\linewidth]{tex/images/app-left-original.png} &
    \includegraphics[height=.4\linewidth]{tex/images/app-left-original.png} &
    \includegraphics[height=.4\linewidth]{tex/images/app-left-original.png} &
    \includegraphics[height=.4\linewidth]{tex/images/app-left-original.png} \\
    \midrule
    \includegraphics[height=.4\linewidth]{tex/images/app-left-original.png} &
    \includegraphics[height=.4\linewidth]{tex/images/app-left-original.png} &
    \includegraphics[height=.4\linewidth]{tex/images/app-left-original.png} & & &
    \includegraphics[height=.4\linewidth]{tex/images/app-left-original.png} &
    \includegraphics[height=.4\linewidth]{tex/images/app-left-original.png} &
    \includegraphics[height=.4\linewidth]{tex/images/app-left-original.png} &
    \includegraphics[height=.4\linewidth]{tex/images/app-left-original.png} \\
    \midrule
    \includegraphics[height=.4\linewidth]{tex/images/app-left-original.png} &
    \includegraphics[height=.4\linewidth]{tex/images/app-left-original.png} &
    \includegraphics[height=.4\linewidth]{tex/images/app-left-original.png} & & &
    \includegraphics[height=.4\linewidth]{tex/images/app-left-original.png} &
    \includegraphics[height=.4\linewidth]{tex/images/app-left-original.png} &
    \includegraphics[height=.4\linewidth]{tex/images/app-left-original.png} &
    \includegraphics[height=.4\linewidth]{tex/images/app-left-original.png} \\
    \end{tabular}
\caption{\textbf{More qualitative comparisons with baseline methods.}
We provide qualitative examples of the translation results produced by various methods. 
% The left-most column shows the input images in the source domain. The other seven columns show the corresponding translated images in the target domain. Every three rows from top to bottom are: dog$\rightarrow$cat, winter$\rightarrow$summer, and photo$\rightarrow$portrait.
% We visualize the unpaired translated results produced by different methods. The left column shows the input images in the source domain. The other seven columns show the corresponding generated images in the target domain. From top to bottom are: dog2cat, winter2summer, and photo2portrait.
}
\label{fig:baseline}
\end{figure*}
